# Supplementary material for: BIM: Block-Wise Self-Supervised Learning with Masked Image Modeling
Source: arXiv:2311.17218 source file (2023-11-28)
Supplement: Supplementary file 1 [file X_suppl.tex]

\clearpage
\setcounter{page}{1}
\maketitlesupplementary
\section{Implementation Details}
In this section, we will provide an in-depth overview of the specific configurations utilized for both the pretraining and finetuning phases of BIM. The code will be made available upon the acceptance of our work.
\subsection{BIM architecture} 
Following the original MAE, we implemented the standard ViT architecture as the backbone architecture. In MAE, it sets the encoder and decoder to have different widths and adopts a linear projection layer to match them. Besides, its encoder also ends with a LayerNorm. Hence, to match this setting, for all blocks in BIM, we assigned the same LayerNorm and linear layer to match them with their identical decoder. Except for this difference, all other architecture settings are the same with raw MAE.

\subsection{Pretraining Settings} 
\label{sec:pretraining-settings}
Before pretraining, following official ViT implementation, we used xavier\_uniform in Pytorch to initialize all Transformer blocks. Besides, we used a conventional linear learning rate ($lr$) scaling rule: $lr=base\_{lr} \times batch\_size/256$. Notably, the batch size is selected from 2048, 4096, and 8192, according to the experiment requirement. Each ViT backbone is pretrained with either 400 epochs or 800 epochs. Other general pretraining configurations are listed in Table~\ref{tab-Petraining-setting}.
\begin{table}[htbp]
\centering
\begin{tabular}{l|l}
\toprule
General Configuration & Detail \\
\midrule
Optimizer & AdamW~\cite{loshchilov2019decoupled} \\
Base Learning Rate & 1.5e-4 \\
Weight Decay & 0.05 \\
Optimizer Momentum & \(\beta_1, \beta_2=0.9, 0.95\)\\
Learning Rate Schedule & cosine decay~\cite{loshchilov2017sgdr} \\
Warmup Epochs~\cite{goyal2018accurate} & 40 \\
Data Augmentation & RandomResizedCrop \\
\bottomrule
\end{tabular}
\caption{General configuration for the pretraining process.}
\label{tab-Petraining-setting}
\end{table}

\subsection{End-to-end Fine-tuning Settings}
\label{sec:finetuning-settings}
The pretrained ViT encoder backbone with BIM are fully-finetuned over ImageNet dataset. The end-to-end fine-tuning training epochs is set to 100 for ViT-base, and 50 for ViT-large and ViT-huge. Besides, the value of the drop path is set to be 0.1, 0.2 and 0.3 for ViT-base, ViT-large and ViT-huge, respectively. Base learning rate is set to 5e-4 for ViT-base and 1e-3 for ViT-large and ViT-huge.
The other general configurations we used are listed in Table \ref{tab-end-finetune-setting}.
\begin{table}[htbp]
\centering
\begin{tabular}{@{}l|l@{}}
\toprule
General Configuration & Detail \\ \midrule
Optimizer & AdamW \\
Weight Decay & 0.05 \\
Optimizer Momentum & $\beta_1, \beta_2=0.9, 0.999$ \\
Layer-wise $lr$ Decay~\cite{clark2020electra} & 0.75 \\
Batch Size & 1024 \\
Learning Rate Schedule & cosine decay \\
Augmentation & RandAug (9, 0.5) \\
Label Smoothing~\cite{szegedy2015rethinking}& 0.1 \\
Mixup~\cite{zhang2018mixup}& 0.8 \\
Cutmix~\cite{yun2019cutmix}& 1.0 \\ \bottomrule
\end{tabular}
\caption{General configuration for the end-to-end fine-tuning process.}
\label{tab-end-finetune-setting}
\end{table}

\subsection{Linear Probing Settings}
Following the linear probing implementation in the original MAE, we disabled many common regularization strategies and set the weight decay to 0. The other general configurations are listed in the Table \ref{tab-linear-probing-setting}.
\begin{table}[htbp]
\centering
\begin{tabular}{@{}l|l@{}}
\toprule
General Configuration          & Detail   \\ \midrule
Optimizer                & LARS~\cite{you2017large}         \\
Base learning rate       & 0.1               \\
Optimizer momentum       & 0.9               \\
Batch size               & 16384             \\
Learning rate schedule   & Cosine decay      \\
Warmup epochs            & 10                \\
Training epochs          & 90                \\
Augmentation             & RandomResizedCrop \\ \bottomrule
\end{tabular}
\caption{General configuration for the linear probing process.}
\label{tab-linear-probing-setting}
\end{table}

\subsection{Settings for Once-for-all BIM Training}
For~\textit{Independent training (IT)}, we employ a procedure where we selectively truncate the ViT encoder backbone to different depths. Subsequently, we conduct MAE pretraining for each of these truncated subnetworks. Following the pretraining phase, we proceed with end-to-end finetuning for each of these pretrained ViT backbones. All ViT backbones are pretrained
for 400 epochs, then fine-tuned with 100 epochs for ViT-base and 50 epochs for ViT-large and ViT-huge. The rest settings align with those elaborated in in Section~\ref{sec:pretraining-settings} and Section~\ref{sec:finetuning-settings}. Following this, we proceed to perform end-to-end fine-tuning for each truncated ViT backbone. Specifically, we employ 100 epochs for ViT-base and 50 epochs for both ViT-large and ViT-huge during the fine-tuning process.

\subsection{Object Detection and Segmentation in COCO}
As we introduced in \ref{sec:exp-implementation}, following ViTDet framework~\cite{li2022exploring}, we adapt the vanilla ViT for the use of an FPN~\cite{lin2017feature} backbone in MaskR-CNN~\cite{he2017mask}. The value of the drop path is 0.1 for ViT-base and 0.4 for ViT-large. Other general configurations are listed in Table~\ref{tab-coco-setting}.
\begin{table}[htbp]
\centering
\begin{tabular}{@{}l|l@{}}
\toprule
General Configuration          & Detail    \\ \midrule
Optimizer                & AdamW             \\
Optimizer Momentum       & $\beta_1, \beta_2=0.9, 0.999$ \\
Warmup Iterations        & 250                \\
Batch size               & 64               \\
Base learning rate       & 0.1               \\
Augmentation             & Large-scale Jitter \\ 
Scale Range              & [0.1,2.0]         \\
Input Size               & $1024 \times 1024$ \\
Learning Rate            & 1e-4             \\
Weight Decay             & 0.1               \\
Epochs                   & 100               \\
\bottomrule
\end{tabular}
\caption{General configuration for the transfer learning in COCO.}
\label{tab-coco-setting}
\end{table}

\subsection{Peak Memory Measurement}
%As the memory pattern during DNN training we introduced in Section~\ref{sec:relatedwork}, the theoretical peak memory consumption can be estimated for the exact input batch size. For our convenience, we used a Python library named \textbf{torch-summary} to obtain the peak GPU memory consumption of MAE and BIM with batch sizes of 2048, 4096, and 8192, separately. Notably, actual peak memory consumption is higher than the estimation values due to the overhead in the Pytorch framework.

We used a Python library \textbf{torch-summary} to obtain the peak GPU memory consumption of MAE and BIM with batch sizes of 2048, 4096, and 8192, separately. 
Torch-summary is a Python library that provides a convenient way to quickly collect the information about a PyTorch neural network model. It allows you to quickly see the peak memory usage during the training process of the model. 

%an overview of the layers, the number of parameters in each layer, and the total number of trainable parameters in the model. 

\begin{comment}
\section{Rationale}
\label{sec:rationale}
% 
Having the supplementary compiled together with the main paper means that:
% 
\begin{itemize}
\item The supplementary can back-reference sections of the main paper, for example, we can refer to \cref{sec:intro};
\item The main paper can forward reference sub-sections within the supplementary explicitly (e.g. referring to a particular experiment); 
\item When submitted to arXiv, the supplementary will already included at the end of the paper.
\end{itemize}
% 
To split the supplementary pages from the main paper, you can use \href{https://support.apple.com/en-ca/guide/preview/prvw11793/mac#:~:text=Delete%20a%20page%20from%20a,or%20choose%20Edit%20%3E%20Delete).}{Preview (on macOS)}, \href{https://www.adobe.com/acrobat/how-to/delete-pages-from-pdf.html#:~:text=Choose%20%E2%80%9CTools%E2%80%9D%20%3E%20%E2%80%9COrganize,or%20pages%20from%20the%20file.}{Adobe Acrobat} (on all OSs), as well as \href{https://superuser.com/questions/517986/is-it-possible-to-delete-some-pages-of-a-pdf-document}{command line tools}.
\end{comment}
